# Supplementary material for: ATiO$_{3}$/TiO (A=Pb, Sn) superlattice: bridging ferroelectricity and conductivity
Source: arXiv:1907.06935 ancillary file (2020-02-10)
Supplement: Supplementary file 1 [file Supplementary.pdf]

# ATiO3/TiO (A=Pb, Sn) superlattice: bridging ferroelectricity and conductivity

S. Raza,[1,2] R. Zhang,[3] N. Zhang,[4] Z. Li,[5] L. Liu,[6] F. Zhang,[1] D. Wang,[1] and C.-L. Jia[1,7]

[1]*School of Microelectronics & State Key Laboratory for Mechanical Behavior of Materials, Xi'an Jiaotong University, Xi'an 710049, China*
[2]*School of Energy and Environment, City University of Hong Kong, Kowloon 999077, Hong Kong Special Administrative Region, China*
[3]*School of Engineering and Materials Science, Queen Mary University of London, London E1 4NS, United Kingdom*
[4]*Electronic Materials Research Laboratory–Key Laboratory of the Ministry of Education and International Center for Dielectric Research, Xi'an Jiaotong University, Xi'an 710049, China*
[5]*School of Materials Science and Engineering, University of Science and Technology Beijing, Beijing 100083, China*
[6]*College of Materials Science and Engineering, Guilin University of Technology, Guilin 541004, China*
[7]*Ernst Ruska Center for Microscopy and Spectroscopy with Electrons, Forschungszentrum, Julich 52425, Germany*

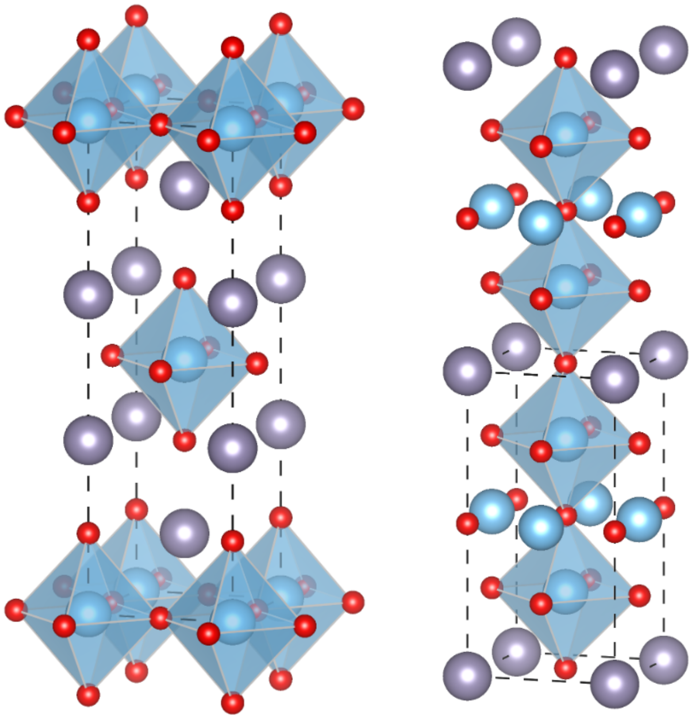

(a) (b)

Figure S1: (a) The crystal structure of the $A_{n+1}Ti_nO_{3n+1}$ (A = Sn) Ruddlesden-Popper (RP) phase. (b) The 1 × 1 × 2 superlattice model of the proposed $ATiO_3$/TiO (A = Sn) structure. The grey, blue, and red spheres represent Sn, Ti, and O atoms, respectively.

| Property | $SnTiO_3$ | $PbTiO_3$ |
|---|---|---|
| a (Å) | 3.78 (3.78) | 3.859 (3.864) |
| c (Å) | 4.28 (4.27) | 4.034 (4.051) |
| c/a (Å) | 1.132 (1.129) | 1.045 (1.048) |
| Polarization ($Cm^{-2}$) | 0.99 (1.1) | 0.76 (0.72) |

Table S1: Optimized structural parameters of tetragonal $SnTiO_3$ and $PbTiO_3$ with the P4mm symmetry. Comparison is established against results from references[1-5]

| Structure | Atoms | $SnTi_4O_7$ | | | $PbTi_4O_7$ | | |
|---|---|---|---|---|---|---|---|
| | | Cm | | Amm2 | Cm | | Amm2 |
| | | Δ x | Δ z | Δ x | Δ x | Δ z | Δ x |
| $ATiO_3$ | A | 0.096 | 0.016 | 0.096 | 0.010 | 0.015 | 0.010 |
| | Ti | 0.023 | 0.004 | 0.025 | 0.018 | 0.001 | 0.018 |
| | O | -0.006 | 0.015 | -0.007 | 0.019 | 0.015 | 0.019 |
| | O | 0.016 | 0.008 | 0.015 | 0.018 | 0.007 | 0.018 |
| | O | 0.002 | 0.008 | 0.006 | 0.021 | 0.007 | 0.021 |
| TiO | Ti | -0.008 | 0.015 | 0.028 | 0.037 | 0.015 | 0.037 |
| | Ti | 0.028 | 0.015 | -0.002 | 0.004 | 0.015 | 0.004 |
| | O | -0.001 | 0.014 | 0.021 | 0.030 | 0.015 | 0.030 |
| | O | 0.030 | 0.015 | -0.003 | 0.003 | 0.015 | 0.002 |
| $TiO_2$ | Ti | 0.023 | 0.026 | 0.025 | 0.018 | 0.028 | 0.018 |
| | O | 0.002 | 0.021 | 0.005 | 0.021 | 0.022 | 0.021 |
| | O | 0.016 | 0.021 | 0.015 | 0.018 | 0.022 | 0.018 |

Table S2: Displacement of atoms (in reduced coordinates) with respect to their ideal positions in the *Cm* and *Amm2* phases. $\Delta x$ and $\Delta z$ represent displacements along the x and z directions, respectively. Note that both the *Cm* and the *Amm2* phases have $\Delta x = \Delta y$ , while the *Amm2* phase further has $\Delta z=0$.

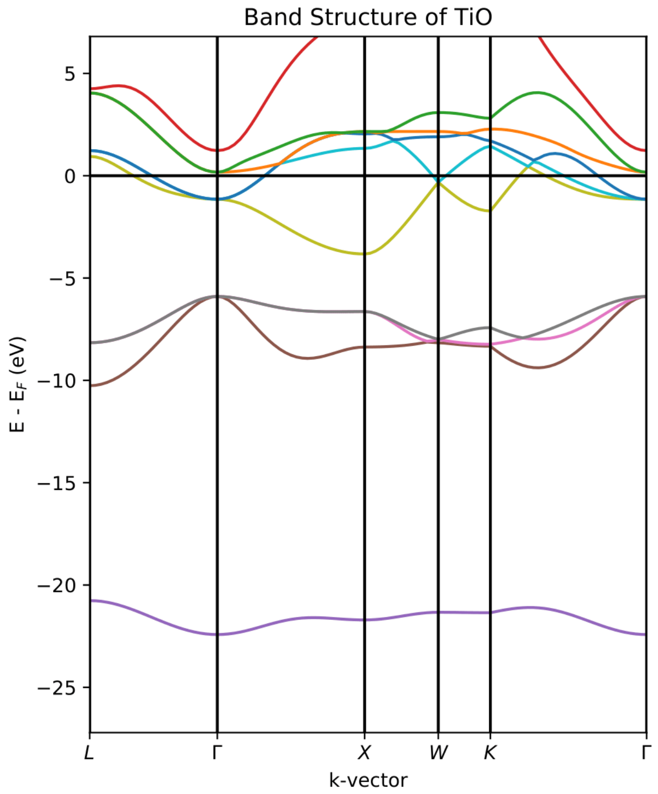


Figure S2: The electronic band structure of TiO.

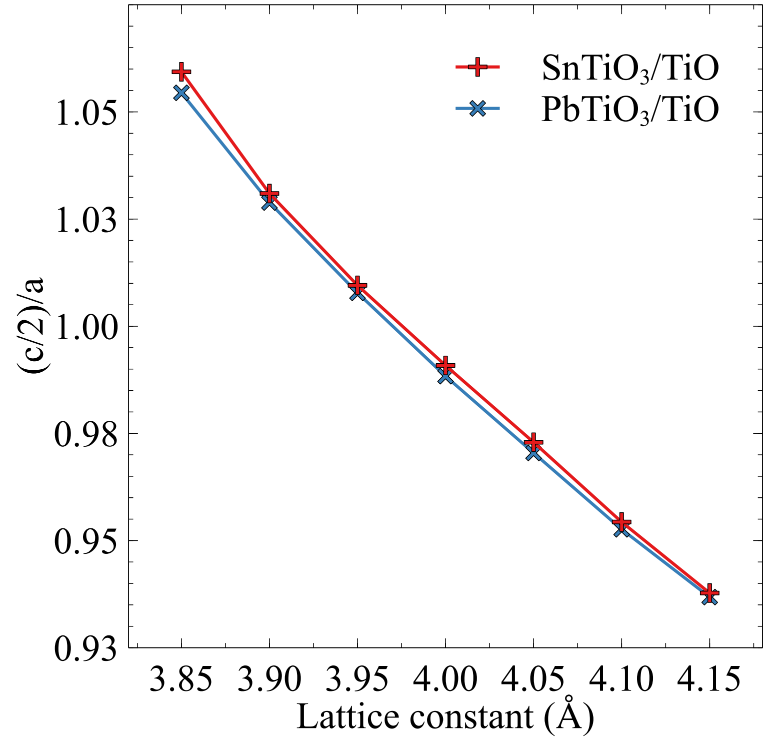


Figure S3: *c/2a* versus the in-plane lattice parameter for $SnTiO_3$/TiO and $PbTiO_3$/TiO.

## References

[1]R. Zhang, D. Wang, X. Zhu, X. Wei, and Z. Xu, *Ruddleson Popper phase SnO($SnTiO_3$)n: Lead-free layered ferroelectric materials with large spontaneous polarization*, J. Appl. Phys. **116**, 174101 (2014).

[2]W. Parker, J. Rondinelli, and S. Nakhmanson, *First-principles study of misfit strain-stabilized ferroelectric $SnTiO_3$*, Phys. Rev. B **84**, 245126 (2011).

[3]Y. Umeno, B. Meyer, C. Elsasser, and P. Gumbsch, *Ab initio study of the critical thickness for ferroelectricity in ultrathin Pt / $PbTiO_3$ /Pt films*, Phys. Rev. B **74**, 060101 (R) (2006).

[4]Y. Xue, D. Chen, Y. Wang, Y. Tang, Y. Zhu, and X. Ma, *The evolution of polarization inside ultrathin PbTiO3 films: a theoretical study*, Philos. Mag **95**, 2067-2077 (2015).

[5]S. Matar, I. Baraille, and M. Subramanian, *First principles studies of $SnTiO_3$ perovskite as potential environmentally benign ferroelectric material*, Chem. Phys. **355**, 43-49 (2009).
